# Supplementary material for: Preference Alignment on Diffusion Model: A Comprehensive Survey for Image Generation and Editing
Source: arXiv:2502.07829 source file (2025-02-10)
Supplement: Supplementary file 1 [file 11_appendix.tex]

\section{Appendix}

\begin{figure}
    \centering
    \includegraphics[width=0.9\linewidth]{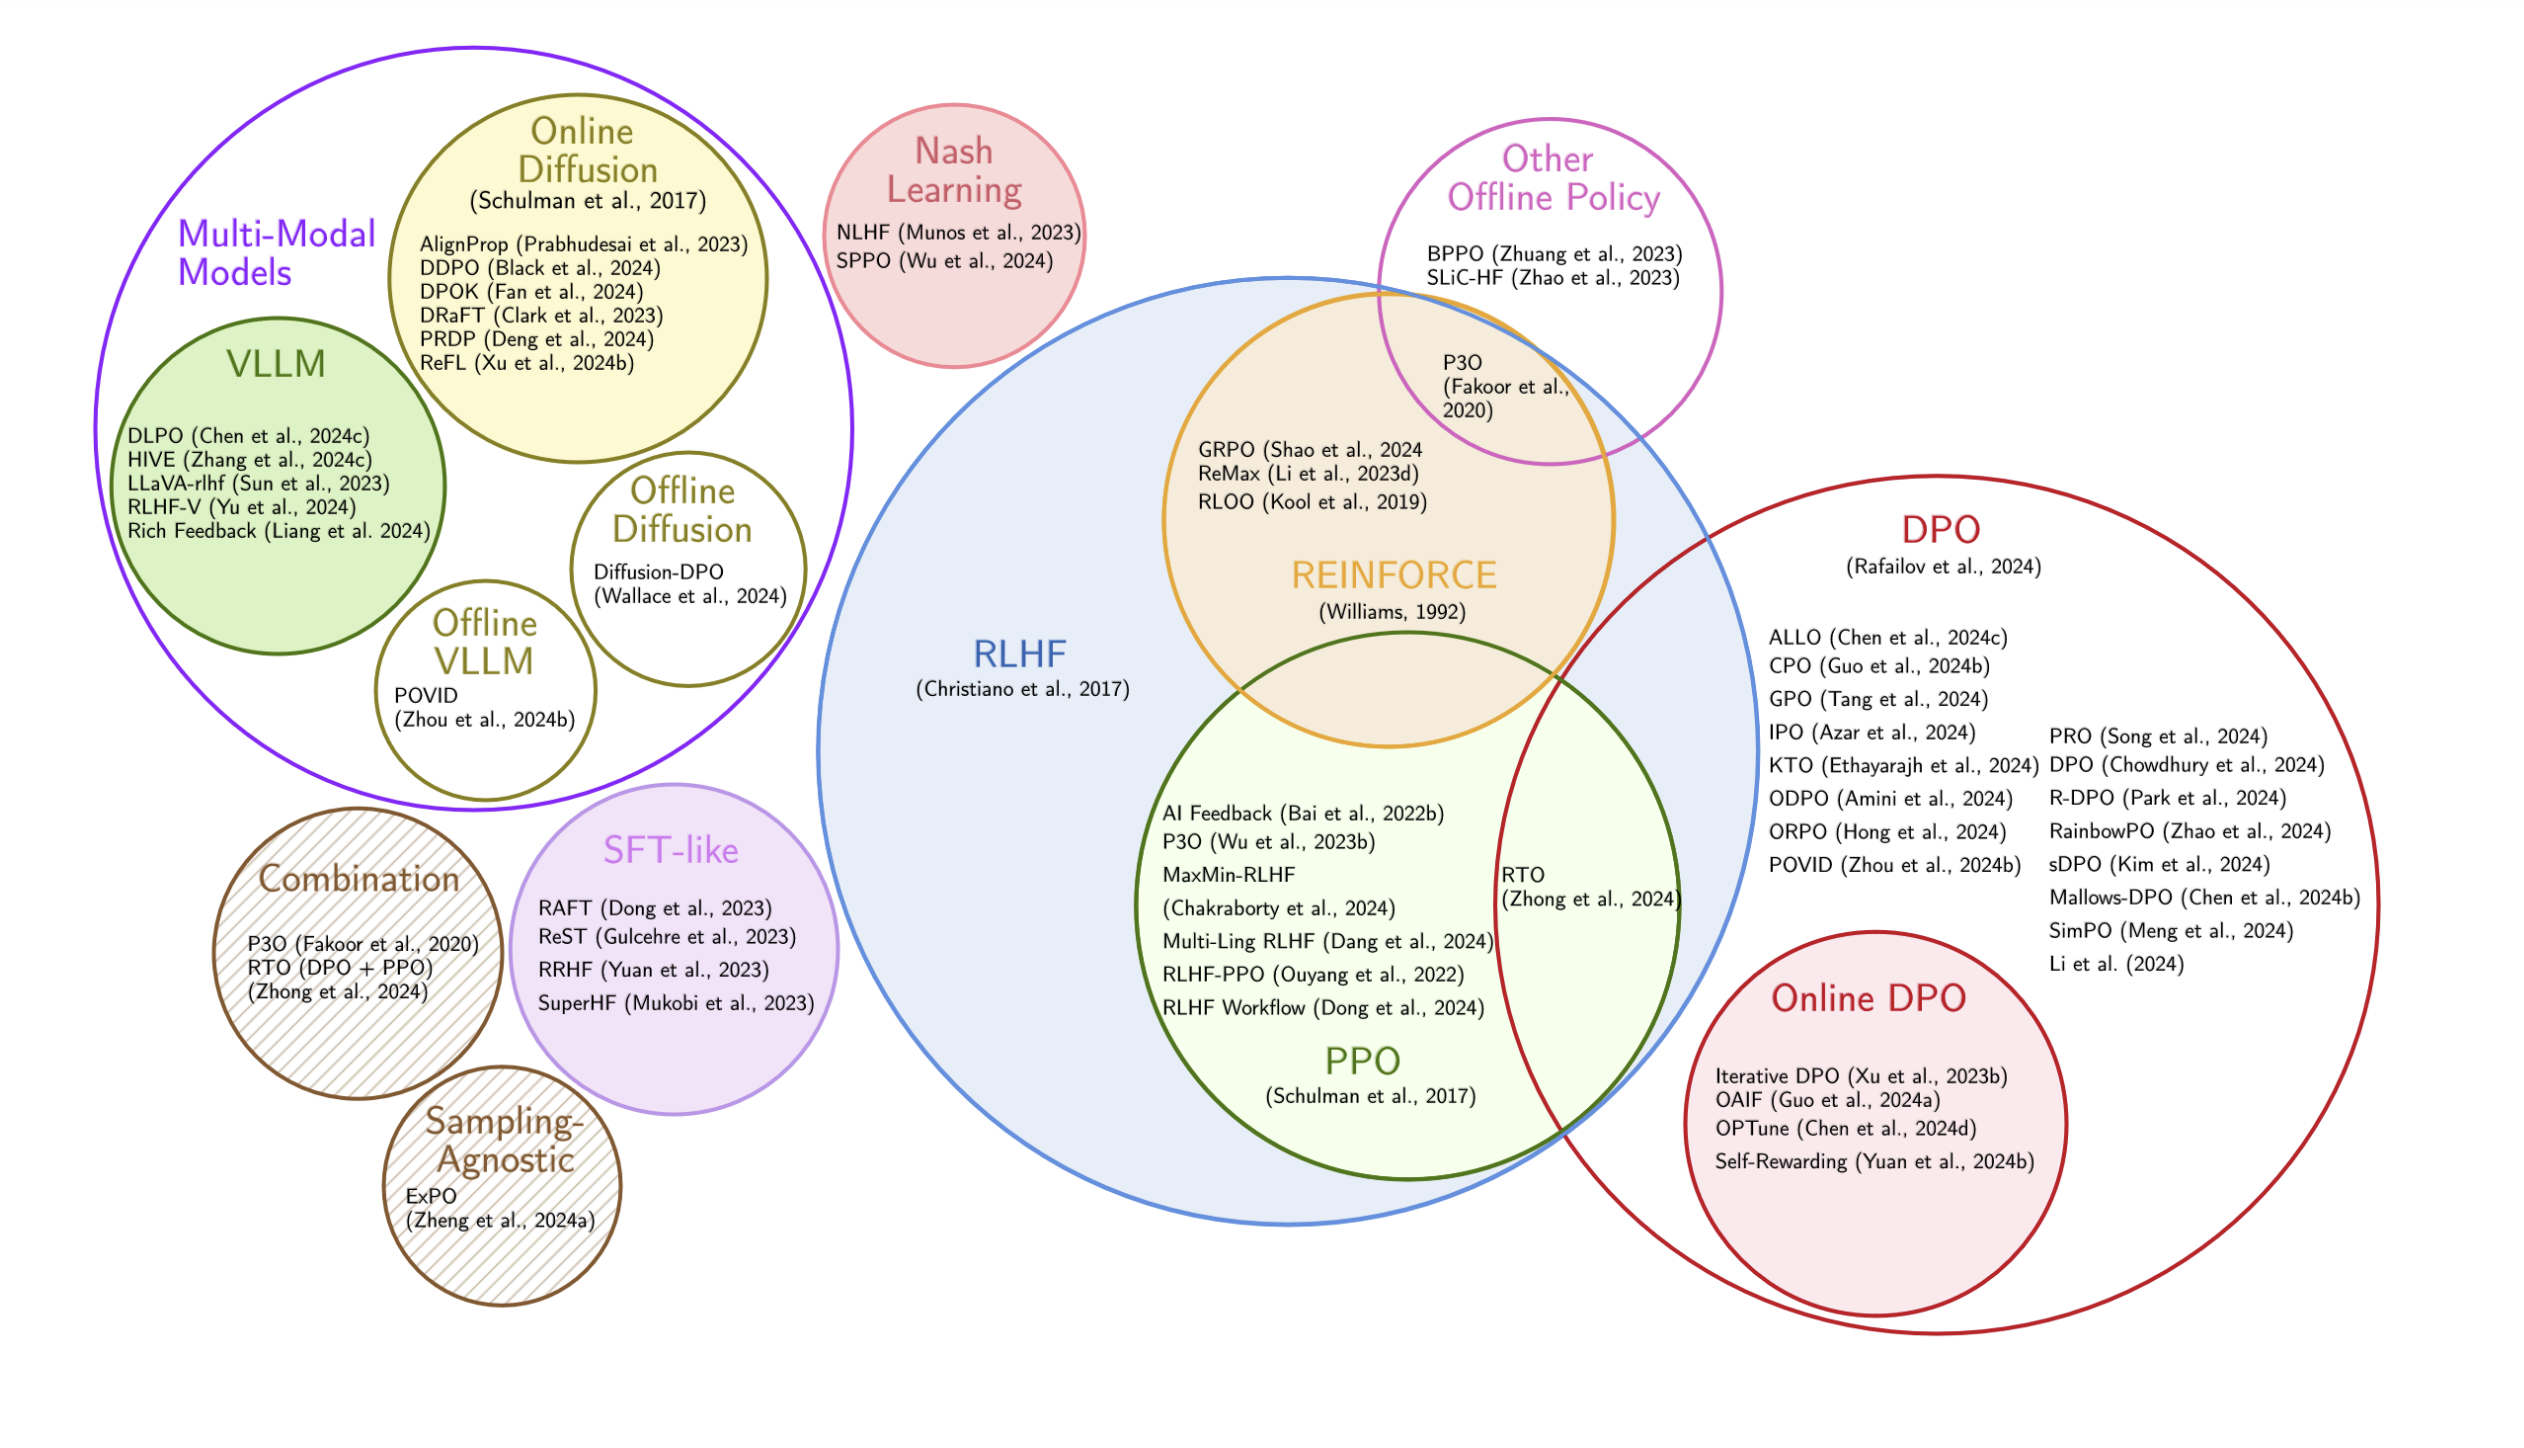}
    \caption{Training Taxonomies}
    \label{fig:traning_taxonomies}
\end{figure}

\begin{figure}
    \centering
    \includegraphics[width=1.0\linewidth]{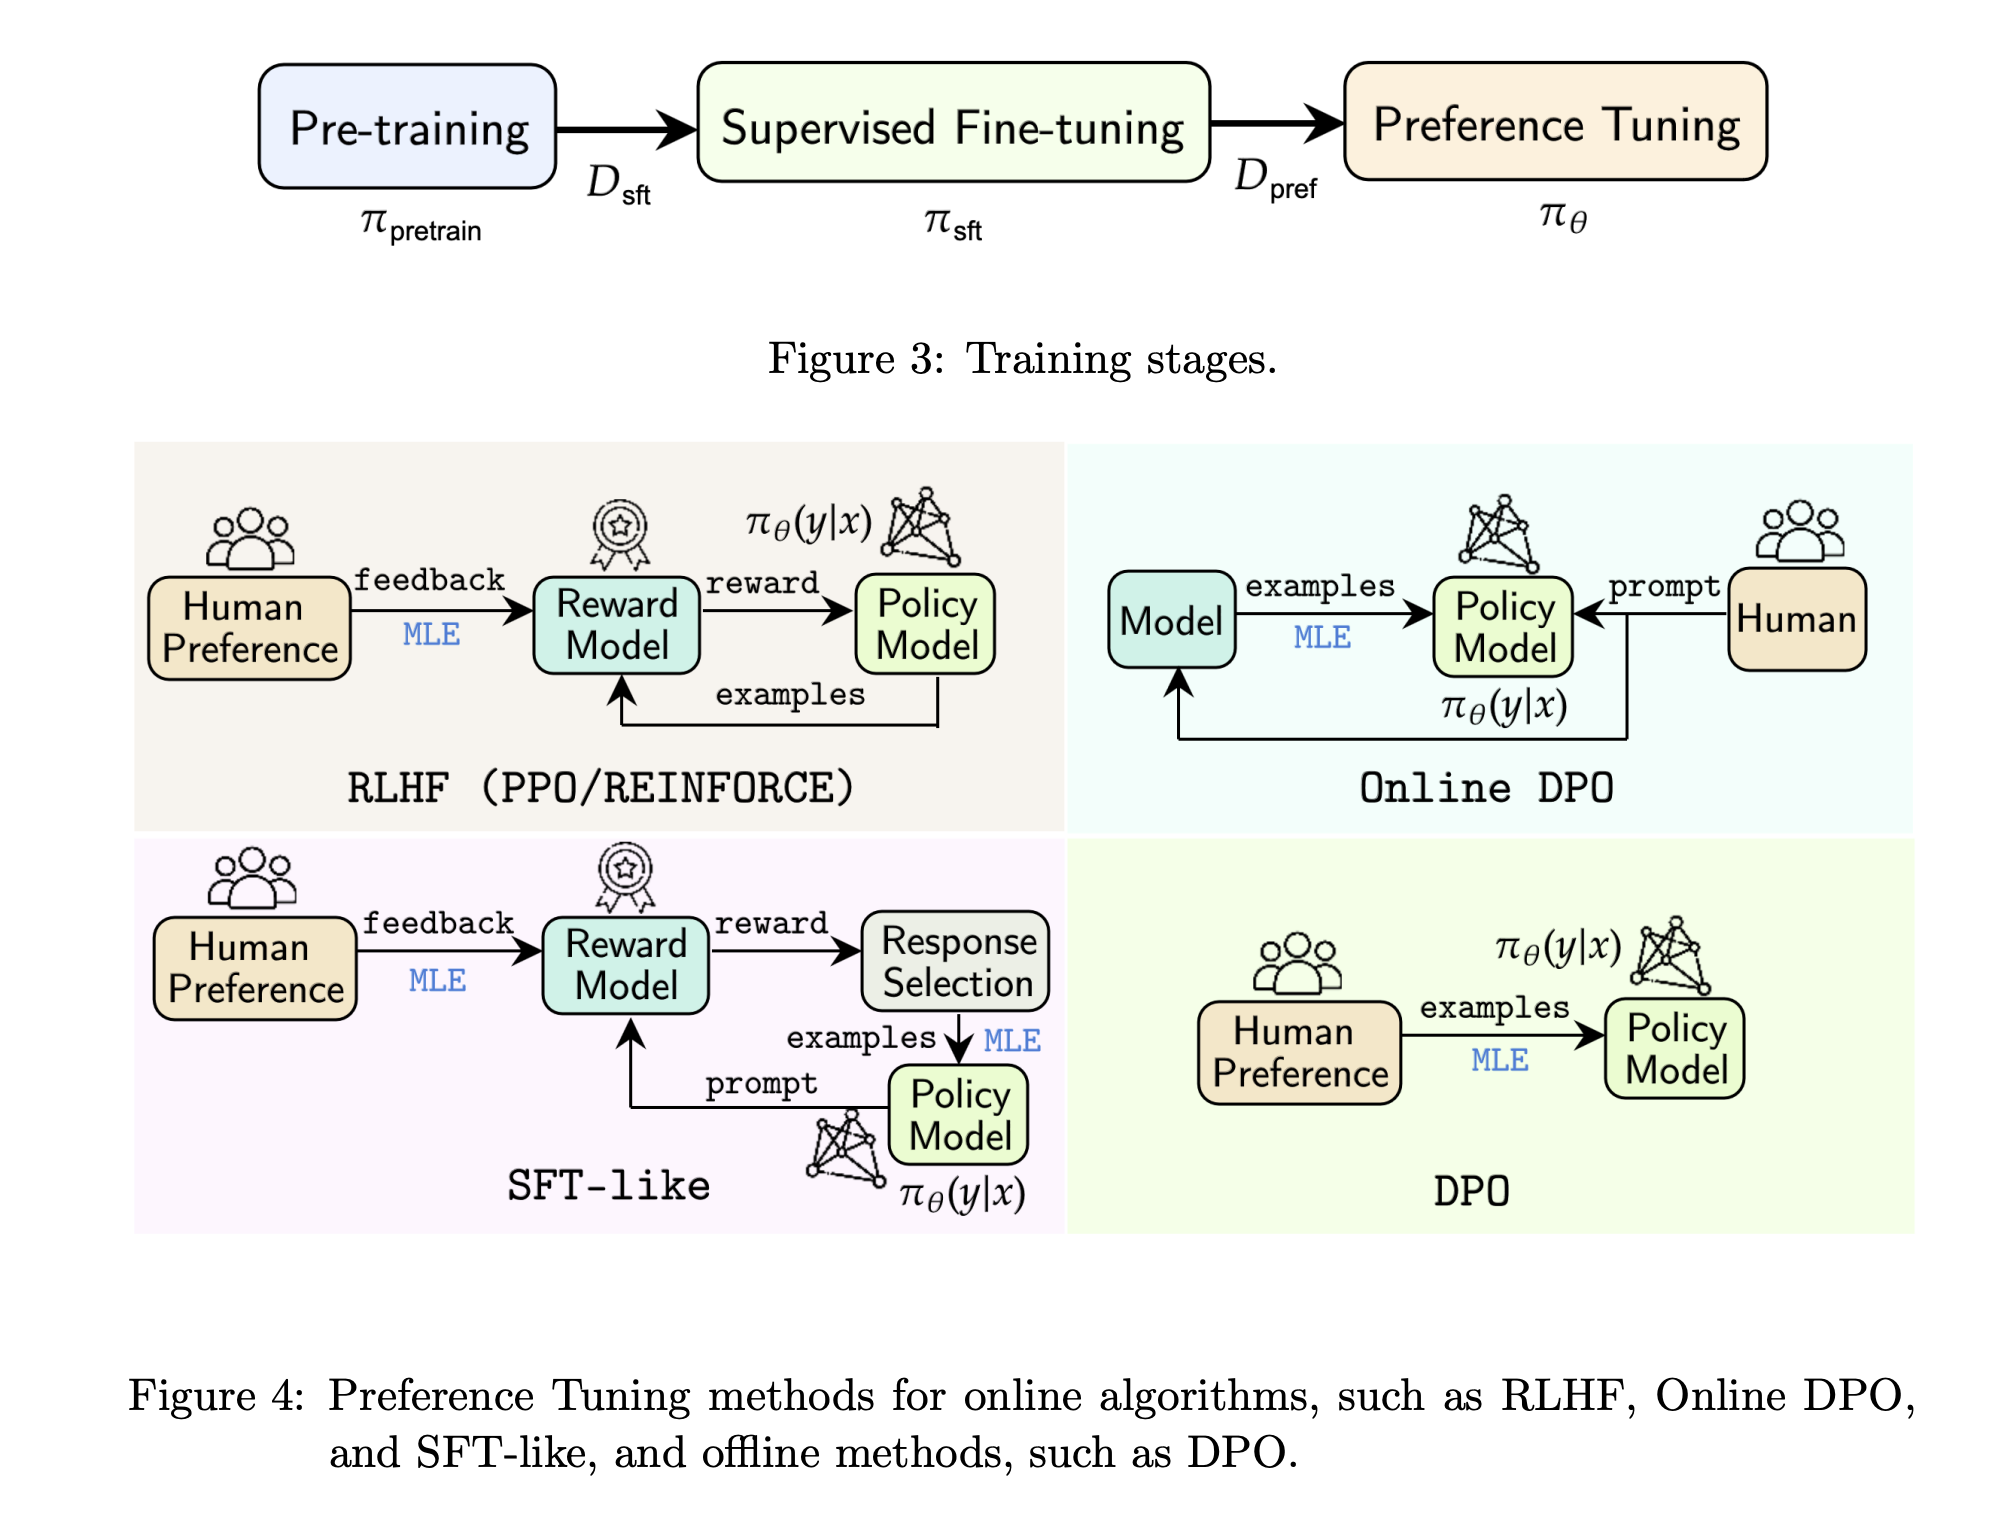}
    \caption{Preference Tuning Taxonomies}
    \label{fig:preference_tuning_taxonogy}
\end{figure}

% \begin{table*}[ht]
%     \centering
%     \input{tables/01_notation}
%     \caption{Caption}
%     \label{tab:notation}
% \end{table*}
